# Supplementary material for: VisionMX: Unlocking Microscaling Post-Training Quantization for Vision Models
Source: arXiv:2610.03218 source file (2026-10-02)
Supplement: Supplementary file 1 [file activation_analysis_appendix.tex]

\paragraph{Layer and samples.}
\autoref{fig:resnet18_relu_fp4_occupancy} reports MXFP4 element-code occupancy for torchvision ResNet18 with pretrained \texttt{IMAGENET1K\_V1} weights.
We capture the second invocation (zero-based index 1) of \texttt{layer4.1.relu}, corresponding to the ReLU after the final residual addition.
The sample set comprises the first lexicographically ordered JPEG in each of the first 16 lexicographically ordered ImageNet validation class directories, using the weights' standard preprocessing.
Each image produces an activation tensor of shape \texttt{[1,512,7,7]}, yielding 401,408 activation values in total.

\paragraph{Quantization and calibration.}
We rearrange the NCHW tensors into spatial-position rows and quantize contiguous groups of 32 channels at each position.
The quantizer uses signed E2M1 elements, dynamically recomputed UE8M0 block scales, TOSA scale calculation, and no clipping.
AAC uses the existing blockwise coordinate-search implementation, fitting a shift and positive affine scale independently for each contiguous 32-channel block.
The objective is reconstruction MSE after quantizing the affine-transformed activations and applying the inverse affine transformation.
The shift and log-scale grids each contain 17 candidates, with two refinements and at most two alternating sweeps.
The search starts from the identity transformation and retains only improvements in reconstruction MSE.

\paragraph{Occupancy and reconstruction error.}
The bars count numeric FP4 element codes after removal of each value's own block scale, rather than raw activations or dequantized values.
The 15 numeric bins combine positive and negative zero; both series include all 401,408 values and sum to 100\%.
\texttt{Raw Data} denotes quantization without affine correction, while \texttt{AAC} denotes quantization in the fitted affine domain.
Each series uses its own dynamic block scales.
The red band marks negative codes, which are unavailable to the nonnegative unshifted ReLU output.
Reconstruction MSE decreases from 0.0505205654 to 0.0288918111, a 42.81\% reduction on the calibration samples.
The same 16 images are used for fitting and plotting, so this is a layer calibration diagnostic rather than a held-out accuracy assessment or a quantized whole-model experiment.
The occupancy counts, sample paths and hashes, fitted parameters, run command, and original script are preserved under \texttt{tools/resnet18\_fp4\_occupancy}.
