# Supplementary material for: VisionMX: Unlocking Microscaling Post-Training Quantization for Vision Models
Source: arXiv:2610.03218 source file (2026-10-02)
Supplement: Supplementary file 2 [file mxfp4_architecture_sensitivity_appendix.tex]

% For a vectorized full-precision weight tensor $\mxWeight$, let $\mxHardWeight=\mxQuantizer(\mxWeight)$ be its quantized tensor.
% Let $V(\mxHardWeight)$ denote the empirical stream of real element codes in $\mxHardWeight$, and let $S(\mxHardWeight)$ denote the empirical stream of stored block-scale codes.
% The local stored scale-code grid for $\mxHardWeight$ is denoted $\mathcal{G}_{s}(\mxHardWeight)$.
% For any discrete stream $\vectorsym{y}$ on code grid $\mathcal{G}$, define
% \[
% \begin{aligned}
% \widehat{p}_{\vectorsym{y}}(a)
% &=
% \frac{|\{y\in \vectorsym{y}:y=a\}|}{|\vectorsym{y}|},
% \\
% H_2(\vectorsym{y};\mathcal{G})
% &=
% -\sum_{a\in\mathcal{G}}
% \widehat{p}_{\vectorsym{y}}(a)\log_2\widehat{p}_{\vectorsym{y}}(a),
% \qquad 0\log_2 0:=0.
% \end{aligned}
% \]
% For weights, effective bit-width is computed per tensor as
% \begin{equation}
% \begin{aligned}
% b_{\mathrm{eff}}
% &=
% H_2(V(\mxHardWeight);\mxFormatSet)
% \\
% &\quad+
% H_2(S(\mxHardWeight);\mathcal{G}_{s}(\mxHardWeight))
% \frac{n_{\mathrm{scale}}}{n_{\mathrm{weight}}},
% \end{aligned}
% \label{eq:weight_effective_bit_width}
% \end{equation}
% where $n_{\mathrm{scale}}$ is the number of stored scale codes and $n_{\mathrm{weight}}$ is the number of real weight parameters in $\mxWeight$.
% The W EBW mean is the parameter-count-weighted mean across quantized weight tensors, and W EBW std is the corresponding weighted population standard deviation.
% EBW is weight-only, uses actual post-BN-fold RTN weight quantization symbols, and was computed with CPU/local-cache model loading without a dataset pass, accuracy rerun, or calibration rerun.
