# Supplementary material for: VisionMX: Unlocking Microscaling Post-Training Quantization for Vision Models
Source: arXiv:2610.03218 source file (2026-10-02)
Supplement: Supplementary file 3 [file mxfp8_architecture_sensitivity_appendix.tex]

As the higher-precision comparison to the MXFP4 sweep, we report the complete 35-model MXFP8 architecture-sensitivity results.
The measurements use separate weight-only and activation-only MXFP8 quantization on ImageNet top-1 accuracy; they do not include joint weight-and-activation quantization or provide a deployment ranking.
The ViT-B-16, Swin-T, DeiT-Tiny, DeiT-Small, and DeiT-Base rows are marked as partial attention coverage in the evaluation logs and are included for completeness, but their transformer attention results should be read as coverage-qualified rather than as full attention quantization results.
All accuracies are ImageNet top-1 percentages, absolute drops are percentage points, and relative losses are percentages relative to the floating-point reference.
For weights, effective bit-width is computed per tensor using \eqref{eq:weight_effective_bit_width}.
The reported W EBW mean is the parameter-count-weighted mean across quantized weight tensors, and W EBW std is the corresponding weighted population standard deviation.
EBW is weight-only, uses actual post-BN-fold RTN weight quantization symbols, and was computed with CPU/local-cache model loading without a dataset pass, accuracy rerun, or calibration rerun.
