# Supplementary material for: VisionMX: Unlocking Microscaling Post-Training Quantization for Vision Models
Source: arXiv:2610.03218 source file (2026-10-02)
Supplement: Supplementary file 4 [file stochastic_block_scale_rounding_appendix.tex]

This appendix documents the diagnostic stochastic block-scale rounding experiment summarized in \autoref{fig:stochastic_block_scale_rounding_accuracy_histogram}.
The experiment studies sensitivity to MX block-scale rounding for weight-only quantization, rather than proposing stochastic scale selection as a deployment method.

\paragraph{Model and data.}
We evaluate the torchvision pretrained ResNet18 on the ImageNet validation set.
The floating-point reference model obtains top-1 accuracy of 0.697600.

\paragraph{Quantization setup.}
The quantized setting is weight-only \texttt{mxfp4}.
Activations remain in floating point, and the default E8/\agentsreplace{E8M0}{UE8M0} block scale is used through \texttt{weight\_block\_scale\_format: null}.
The main-flow RTN baseline obtains top-1 accuracy of 0.645380 under this setup.

\paragraph{Stochastic block-scale rounding policy.}
For each non-exact scale position, the stochastic policy chooses the lower or upper adjacent representable scale with probabilities proportional to the floating-point scale position between those adjacent representable scales.
Exact scale hits are tracked separately.
This policy is applied only to measure sensitivity to block-scale rounding choices in the weight-only MXFP4 configuration.

\paragraph{Trials and summary.}
We run $K=100$ stochastic trials with seeds 0 through 99.
Across these trials, top-1 accuracy has mean 0.636179, standard deviation 0.0050745, minimum 0.62532, and maximum 0.64790.
The observed spread shows that block-scale rounding can be a non-negligible contributor to accuracy variation in this configuration, while the mean being below the deterministic RTN baseline cautions against interpreting stochastic scale rounding as an improved quantization recipe.

\paragraph{Provenance.}
The 100 stochastic trials and histogram inputs are stored in the code repository at \path{results/stochastic_block_scale_rounding/results.json}.
The main-flow RTN baseline of 0.645380 is stored at \path{results/resnet18_mxfp4_e8_mainflow_rtn/results.json}.
The runner is \path{analysis/run_stochastic_block_scale_rounding.py}, the plot script is \path{analysis/plot_stochastic_block_scale_results.py}, and the preserved SVG under \path{figure/} has a PDF derivative used for \texttt{pdflatex} compilation.
